# Supplementary material for: Local self-interaction correction method with a simple scaling factor
Source: arXiv:2010.08921 source file (2020-10-18)
Supplement: Supplementary file 1 [file SI.pdf]

# Supplemental information for: Local self-interaction correction method with a simple scaling factor

Selim Romero[1,2], Yoh Yamamoto[1], Tunna Baruah[1,2], and Rajendra Zope[1,2]

[1]Department of Physics, University of Texas at El Paso, El Paso, Texas 79968, USA
[2]Computational Science Program, University of Texas at El Paso, El Paso, Texas 79968, USA

October 13, 2020

**Table S1** Total energies of atoms (in Ha) for PZSIC, LSIC($z$), and LSIC($w$) with varying values in $k$ using LSDA.

| $Z$ | PZSIC | LSIC($z$) | LSIC($w$) | | | | $E^{\dagger}_{Accu}$ |
|---|---|---|---|---|---|---|---|
| | | $k=1$ | $k=1$ | $k=2$ | $k=3$ | $k=4$ | |
| 1 | -0.500 | -0.500 | -0.500 | -0.500 | -0.500 | -0.500 | -0.500 |
| 2 | -2.920 | -2.920 | -2.920 | -2.920 | -2.920 | -2.920 | -2.904 |
| 3 | -7.509 | -7.501 | -7.503 | -7.500 | -7.498 | -7.496 | -7.478 |
| 4 | -14.707 | -14.678 | -14.687 | -14.678 | -14.671 | -14.666 | -14.667 |
| 5 | -24.726 | -24.670 | -24.681 | -24.660 | -24.646 | -24.635 | -24.654 |
| 6 | -37.955 | -37.867 | -37.869 | -37.833 | -37.809 | -37.792 | -37.845 |
| 7 | -54.741 | -54.615 | -54.603 | -54.550 | -54.518 | -54.495 | -54.589 |
| 8 | -75.285 | -75.101 | -75.085 | -75.007 | -74.959 | -74.923 | -75.067 |
| 9 | -100.012 | -99.768 | -99.729 | -99.621 | -99.554 | -99.507 | -99.734 |
| 10 | -129.281 | -128.971 | -128.906 | -128.769 | -128.687 | -128.630 | -128.938 |
| 11 | -162.673 | -162.273 | -162.210 | -162.045 | -161.948 | -161.881 | -162.255 |
| 12 | -200.548 | -200.046 | -199.993 | -199.800 | -199.688 | -199.612 | -200.053 |
| 13 | -242.920 | -242.323 | -242.270 | -242.047 | -241.919 | -241.832 | -242.346 |
| 14 | -290.010 | -289.313 | -289.260 | -289.007 | -288.864 | -288.767 | -289.359 |
| 15 | -341.982 | -341.185 | -341.130 | -340.847 | -340.689 | -340.583 | -341.259 |
| 16 | -398.929 | -398.018 | -397.968 | -397.653 | -397.477 | -397.359 | -398.110 |
| 17 | -461.059 | -460.032 | -459.983 | -459.634 | -459.442 | -459.314 | -460.148 |
| 18 | -528.539 | -527.396 | -527.344 | -526.964 | -526.756 | -526.618 | -527.540 |
| 19 | -601.004 | -599.732 | -599.695 | -599.284 | -599.061 | -598.914 | |
| 20 | -678.752 | -677.340 | -677.321 | -676.878 | -676.639 | -676.483 | |
| 21 | -761.957 | -760.388 | -760.375 | -759.891 | -759.632 | -759.463 | |
| 22 | -850.866 | -849.128 | -849.127 | -848.602 | -848.322 | -848.140 | |
| 23 | -945.513 | -943.637 | -943.624 | -943.070 | -942.777 | -942.588 | |
| 24 | -1046.123 | -1044.167 | -1044.119 | -1043.548 | -1043.249 | -1043.056 | |
| 25 | -1152.838 | -1150.693 | -1150.653 | -1150.042 | -1149.727 | -1149.525 | |
| 26 | -1265.725 | -1263.386 | -1263.355 | -1262.701 | -1262.364 | -1262.149 | |
| 27 | -1385.019 | -1382.468 | -1382.458 | -1381.756 | -1381.396 | -1381.165 | |
| 28 | -1510.546 | -1507.950 | -1507.897 | -1507.191 | -1506.833 | -1506.606 | |
| 29 | -1642.968 | -1640.180 | -1640.085 | -1639.344 | -1638.975 | -1638.743 | |
| 30 | -1782.107 | -1779.074 | -1779.009 | -1778.220 | -1777.828 | -1777.582 | |
| 31 | -1927.727 | -1924.467 | -1924.428 | -1923.589 | -1923.174 | -1922.915 | |
| 32 | -2080.027 | -2076.542 | -2076.527 | -2075.642 | -2075.205 | -2074.933 | |
| 33 | -2239.101 | -2235.395 | -2235.403 | -2234.473 | -2234.015 | -2233.731 | |
| 34 | -2404.970 | -2401.038 | -2401.072 | -2400.096 | -2399.617 | -2399.319 | |
| 35 | -2577.773 | -2573.616 | -2573.671 | -2572.650 | -2572.150 | -2571.841 | |
| 36 | -2757.608 | -2753.224 | -2753.301 | -2752.237 | -2751.717 | -2751.396 | |
| MAE | 0.381 | 0.041 | 0.061 | 0.196 | 0.277 | 0.332 | |

†Reference [1]

**Table S2** Total energies of atoms (in Ha) for OSIC($w$) with varying values in $k$ using LSDA.

| $Z$ | OSIC($w$) | | | $E^{\dagger}_{Accu}$ |
|---|---|---|---|---|
| | $k=1$ | $k=2$ | $k=3$ | |
| 1 | -0.500 | -0.500 | -0.500 | -0.500 |
| 2 | -2.920 | -2.920 | -2.920 | -2.904 |
| 3 | -7.506 | -7.504 | -7.503 | -7.478 |
| 4 | -14.696 | -14.690 | -14.686 | -14.667 |
| 5 | -24.700 | -24.687 | -24.677 | -24.654 |
| 6 | -37.902 | -37.876 | -37.858 | -37.845 |
| 7 | -54.651 | -54.611 | -54.585 | -54.589 |
| 8 | -75.155 | -75.095 | -75.056 | -75.067 |
| 9 | -99.821 | -99.736 | -99.681 | -99.734 |
| 10 | -129.023 | -128.912 | -128.842 | -128.938 |
| 11 | -162.346 | -162.208 | -162.124 | -162.255 |
| 12 | -200.151 | -199.987 | -199.888 | -200.053 |
| 13 | -242.451 | -242.260 | -242.146 | -242.346 |
| 14 | -289.464 | -289.245 | -289.115 | -289.359 |
| 15 | -341.358 | -341.111 | -340.964 | -341.259 |
| 16 | -398.223 | -397.945 | -397.782 | -398.110 |
| 17 | -460.264 | -459.954 | -459.774 | -460.148 |
| 18 | -527.652 | -527.310 | -527.112 | -527.540 |
| 19 | -600.028 | -599.656 | -599.442 | |
| 20 | -677.684 | -677.280 | -677.049 | |
| 21 | -760.782 | -760.339 | -760.085 | |
| 22 | -849.576 | -849.092 | -848.815 | |
| 23 | -944.113 | -943.596 | -943.303 | |
| 24 | -1044.646 | -1044.106 | -1043.801 | |
| 25 | -1151.220 | -1150.639 | -1150.313 | |
| 26 | -1263.976 | -1263.350 | -1262.998 | |
| 27 | -1383.129 | -1382.455 | -1382.077 | |
| 28 | -1508.602 | -1507.919 | -1507.539 | |
| 29 | -1640.861 | -1640.134 | -1639.734 | |
| 30 | -1779.822 | -1779.042 | -1778.615 | |
| 31 | -1925.275 | -1924.445 | -1923.993 | |
| 32 | -2077.411 | -2076.534 | -2076.057 | |
| 33 | -2236.324 | -2235.399 | -2234.899 | |
| 34 | -2402.033 | -2401.061 | -2400.536 | |
| 35 | -2574.673 | -2573.654 | -2573.106 | |
| 36 | -2754.345 | -2753.279 | -2752.706 | |
| MAE | 0.074 | 0.070 | 0.135 | |

†Reference [1]

**Table S3** Δ-SCF ionization potentials (in eV) for PZSIC, LSIC($z$), and LSIC($w,k$) where $k = 1-4$ with LSDA.

| $Z$ | PZSIC | LSIC($z$) | LSIC($w$) | | | | $E^{\dagger}_{Exp}$ |
|---|---|---|---|---|---|---|---|
| | | $k=1$ | $k=1$ | $k=2$ | $k=3$ | $k=4$ | |
| 2 | 25.032 | 25.032 | 25.032 | 25.032 | 25.032 | 25.032 | 24.587 |
| 3 | 5.539 | 5.307 | 5.373 | 5.292 | 5.237 | 5.194 | 5.392 |
| 4 | 9.195 | 8.881 | 8.989 | 8.881 | 8.806 | 8.748 | 9.323 |
| 5 | 8.940 | 8.698 | 8.567 | 8.394 | 8.274 | 8.179 | 8.298 |
| 6 | 11.628 | 11.516 | 11.047 | 10.860 | 10.763 | 10.702 | 11.260 |
| 7 | 14.716 | 14.747 | 14.188 | 14.114 | 14.102 | 14.104 | 14.534 |
| 8 | 14.300 | 14.011 | 13.864 | 13.612 | 13.418 | 13.256 | 13.618 |
| 9 | 17.598 | 17.511 | 16.815 | 16.541 | 16.394 | 16.297 | 17.423 |
| 10 | 21.525 | 21.651 | 20.881 | 20.804 | 20.803 | 20.817 | 21.565 |
| 11 | 5.360 | 4.992 | 5.204 | 5.216 | 5.240 | 5.262 | 5.139 |
| 12 | 7.787 | 7.363 | 7.593 | 7.596 | 7.617 | 7.638 | 7.646 |
| 13 | 6.204 | 6.143 | 6.066 | 6.010 | 5.972 | 5.943 | 5.986 |
| 14 | 8.190 | 8.183 | 8.010 | 7.976 | 7.968 | 7.968 | 8.152 |
| 15 | 10.409 | 10.483 | 10.268 | 10.279 | 10.298 | 10.316 | 10.487 |
| 16 | 10.826 | 10.644 | 10.631 | 10.569 | 10.530 | 10.499 | 10.360 |
| 17 | 13.174 | 13.074 | 12.885 | 12.830 | 12.819 | 12.820 | 12.968 |
| 18 | 15.803 | 15.837 | 15.575 | 15.579 | 15.603 | 15.629 | 15.760 |
| 19 | 4.459 | 4.150 | 4.335 | 4.355 | 4.383 | 4.408 | 4.341 |
| 20 | 6.184 | 5.835 | 6.021 | 6.036 | 6.064 | 6.091 | 6.113 |
| 21 | 7.596 | 6.838 | 6.763 | 6.689 | 6.702 | 6.728 | 6.561 |
| 22 | 8.170 | 7.036 | 7.686 | 7.665 | 7.701 | 7.743 | 6.828 |
| 23 | 6.277 | 6.734 | 6.397 | 6.725 | 6.998 | 7.213 | 6.746 |
| 24 | 7.018 | 6.920 | 6.988 | 7.109 | 7.182 | 7.227 | 6.767 |
| 25 | 7.511 | 7.103 | 6.922 | 6.946 | 7.033 | 7.117 | 7.434 |
| 26 | 8.928 | 7.967 | 8.046 | 7.960 | 7.972 | 8.000 | 7.902 |
| 27 | 8.265 | 7.793 | 7.946 | 7.967 | 8.022 | 8.083 | 7.881 |
| 28 | 5.083 | 7.806 | 6.601 | 7.442 | 7.990 | 8.372 | 7.640 |
| 29 | 7.770 | 7.672 | 7.771 | 7.946 | 8.052 | 8.119 | 7.726 |
| 30 | 9.561 | 9.137 | 9.302 | 9.403 | 9.477 | 9.528 | 9.394 |
| 31 | 6.164 | 6.010 | 6.072 | 6.069 | 6.066 | 6.063 | 5.999 |
| 32 | 7.882 | 7.799 | 7.768 | 7.779 | 7.791 | 7.802 | 7.899 |
| 33 | 9.864 | 9.800 | 9.794 | 9.817 | 9.836 | 9.852 | 9.789 |
| 34 | 10.080 | 9.854 | 9.906 | 9.890 | 9.882 | 9.874 | 9.752 |
| 35 | 12.001 | 11.856 | 11.793 | 11.788 | 11.797 | 11.808 | 11.814 |
| 36 | 14.219 | 14.103 | 14.062 | 14.072 | 14.089 | 14.105 | 14.000 |
| MAE (17 IPs) | 0.248 | 0.206 | 0.251 | 0.271 | 0.297 | 0.324 | |
| MAE (35 IPs) | 0.364 | 0.170 | 0.238 | 0.216 | 0.247 | 0.284 | |

†Reference [2]

**Table S4** Δ-SCF ionization potentials (in eV) for OSIC($w,k$) where $k = 1-3$ with LSDA.

| $Z$ | OSIC($w$) | | | $E^{\dagger}_{Exp}$ |
|---|---|---|---|---|
| | $k=1$ | $k=2$ | $k=3$ | |
| 2 | 25.032 | 25.032 | 25.032 | 24.587 |
| 3 | 5.454 | 5.409 | 5.376 | 5.392 |
| 4 | 9.076 | 9.009 | 8.959 | 9.323 |
| 5 | 8.730 | 8.613 | 8.525 | 8.298 |
| 6 | 11.216 | 11.044 | 10.946 | 11.26 |
| 7 | 14.389 | 14.300 | 14.274 | 14.534 |
| 8 | 14.161 | 14.025 | 13.901 | 13.618 |
| 9 | 17.101 | 16.881 | 16.749 | 17.423 |
| 10 | 21.188 | 21.108 | 21.095 | 21.565 |
| 11 | 5.316 | 5.318 | 5.322 | 5.139 |
| 12 | 7.717 | 7.714 | 7.718 | 7.646 |
| 13 | 6.149 | 6.125 | 6.108 | 5.986 |
| 14 | 8.077 | 8.033 | 8.011 | 8.152 |
| 15 | 10.329 | 10.310 | 10.309 | 10.487 |
| 16 | 10.770 | 10.747 | 10.728 | 10.36 |
| 17 | 12.984 | 12.918 | 12.888 | 12.968 |
| 18 | 15.659 | 15.629 | 15.628 | 15.76 |
| 19 | 4.444 | 4.453 | 4.462 | 4.341 |
| 20 | 6.155 | 6.165 | 6.176 | 6.113 |
| 21 | 7.182 | 7.100 | 7.068 | 6.561 |
| 22 | 7.835 | 7.786 | 7.788 | 6.828 |
| 23 | 6.412 | 6.619 | 6.811 | 6.746 |
| 24 | 7.165 | 7.231 | 7.265 | 6.767 |
| 25 | 7.246 | 7.258 | 7.289 | 7.434 |
| 26 | 8.499 | 8.402 | 8.358 | 7.902 |
| 27 | 8.172 | 8.162 | 8.165 | 7.881 |
| 28 | 6.761 | 7.567 | 8.060 | 7.64 |
| 29 | 7.946 | 8.038 | 8.088 | 7.726 |
| 30 | 9.515 | 9.497 | 9.482 | 9.394 |
| 31 | 6.131 | 6.131 | 6.130 | 5.999 |
| 32 | 7.860 | 7.865 | 7.872 | 7.899 |
| 33 | 9.853 | 9.856 | 9.863 | 9.789 |
| 34 | 10.031 | 10.028 | 10.022 | 9.752 |
| 35 | 11.922 | 11.918 | 11.923 | 11.814 |
| 36 | 14.148 | 14.142 | 14.150 | 14 |
| MAE (17 IPs) | 0.223 | 0.247 | 0.255 | |
| MAE (35 IPs) | 0.267 | 0.247 | 0.259 | |

$^{\dagger}$Reference [2]

**Table S5** Δ-SCF electron affinities (in eV) for PZSIC, LSIC($z$), and LSIC($w,k$) where $k = 1-4$ with LSDA.

| $Z$ | PZSIC | LSIC($z$) | LSIC($w$) | | | | $E_{Exp}^{\dagger}$ |
|---|---|---|---|---|---|---|---|
| | | $k=1$ | $k=1$ | $k=2$ | $k=3$ | $k=4$ | |
| 1 | 0.715 | 0.715 | 0.715 | 0.715 | 0.715 | 0.715 | 0.754 |
| 3 | 0.553 | 0.490 | 0.491 | 0.450 | 0.420 | 0.395 | 0.618 |
| 5 | 0.235 | 0.425 | 0.027 | -0.013 | -0.024 | -0.027 | 0.280 |
| 6 | 1.114 | 1.418 | 0.984 | 1.026 | 1.068 | 1.102 | 1.262 |
| 8 | 1.065 | 1.360 | 0.737 | 0.640 | 0.594 | 0.565 | 1.462 |
| 9 | 2.888 | 3.376 | 2.716 | 2.785 | 2.855 | 2.913 | 3.401 |
| 11 | 0.582 | 0.470 | 0.533 | 0.534 | 0.540 | 0.548 | 0.548 |
| 13 | 0.312 | 0.479 | 0.294 | 0.310 | 0.327 | 0.343 | 0.434 |
| 14 | 1.236 | 1.443 | 1.247 | 1.296 | 1.332 | 1.358 | 1.390 |
| 15 | 0.917 | 0.964 | 0.859 | 0.830 | 0.807 | 0.788 | 0.747 |
| 16 | 2.061 | 2.166 | 1.954 | 1.950 | 1.964 | 1.980 | 2.077 |
| 17 | 3.490 | 3.696 | 3.439 | 3.486 | 3.530 | 3.566 | 3.613 |
| 19 | 0.540 | 0.425 | 0.480 | 0.484 | 0.493 | 0.503 | 0.501 |
| 22 | -1.247 | -0.080 | -1.097 | -0.786 | -0.561 | -0.400 | 0.087 |
| 29 | 1.312 | 1.123 | 1.181 | 1.260 | 1.316 | 1.354 | 1.236 |
| 31 | 0.178 | 0.302 | 0.261 | 0.286 | 0.300 | 0.311 | 0.43 |
| 32 | 1.208 | 1.297 | 1.273 | 1.312 | 1.336 | 1.352 | 1.233 |
| 33 | 0.969 | 0.956 | 0.922 | 0.920 | 0.915 | 0.910 | 0.814 |
| 34 | 2.068 | 2.089 | 1.985 | 1.999 | 2.015 | 2.028 | 2.021 |
| 35 | 3.405 | 3.479 | 3.406 | 3.453 | 3.484 | 3.505 | 3.364 |
| MAE (12 EAs) | 0.152 | 0.097 | 0.235 | 0.229 | 0.215 | 0.202 | |
| MAE (20 EAs) | 0.190 | 0.102 | 0.224 | 0.205 | 0.189 | 0.176 | |

† Reference [3]

**Table S6** $\Delta$-SCF electron affinities (in eV) for OSIC($w,k$) where $k = 1-3$ with LSDA.

| $Z$ | OSIC($w$) | | | $E^{\dagger}_{Exp}$ |
|---|---|---|---|---|
| | $k = 1$ | $k = 2$ | $k = 3$ | |
| 1 | 0.715 | 0.715 | 0.715 | 0.754 |
| 3 | 0.519 | 0.498 | 0.481 | 0.618 |
| 5 | 0.165 | 0.134 | 0.120 | 0.280 |
| 6 | 1.137 | 1.165 | 1.194 | 1.262 |
| 8 | 0.998 | 0.944 | 0.908 | 1.462 |
| 9 | 2.996 | 3.062 | 3.120 | 3.401 |
| 11 | 0.563 | 0.562 | 0.564 | 0.548 |
| 13 | 0.333 | 0.343 | 0.352 | 0.434 |
| 14 | 1.289 | 1.314 | 1.333 | 1.390 |
| 15 | 0.962 | 0.976 | 0.982 | 0.747 |
| 16 | 2.035 | 2.026 | 2.025 | 2.077 |
| 17 | 3.511 | 3.530 | 3.552 | 3.613 |
| 19 | 0.531 | 0.533 | 0.536 | 0.501 |
| 22 | -0.871 | -0.653 | -0.495 | 0.087 |
| 29 | 1.278 | 1.258 | 1.242 | 1.236 |
| 31 | 0.298 | 0.328 | 0.345 | 0.43 |
| 32 | 1.299 | 1.330 | 1.349 | 1.233 |
| 33 | 1.014 | 1.039 | 1.050 | 0.814 |
| 34 | 2.100 | 2.121 | 2.137 | 2.021 |
| 35 | 3.477 | 3.517 | 3.545 | 3.364 |
| MAE (12 EAs) | 0.152 | 0.150 | 0.145 | |
| MAE (20 EAs) | 0.172 | 0.164 | 0.155 | |

$^{\dagger}$Reference [3]

**Table S7** Atomization energies of selected molecules (in kJ/mol) for PZSIC, LSIC($z$), and LSIC($w$).

| System | PZSIC | LSIC($z$) | LSIC($w$) | | | | $E^{\dagger}_{Exp}$ |
|---|---|---|---|---|---|---|---|
| | | $k=1$ | $k=1$ | $k=2$ | $k=3$ | $k=4$ | |
| HF | 609.4 | 603.6 | 568.7 | 562.7 | 560.4 | 559.0 | 566.6 |
| LiF | 558.1 | 557.6 | 513.7 | 509.4 | 507.8 | 506.1 | 575.6 |
| $F_2$ | 189.9 | 150.8 | 204.8 | 222.2 | 230.9 | 235.7 | 154.5 |
| HCl | 490.4 | 460.5 | 455.8 | 447.1 | 442.6 | 439.6 | 427.8 |
| LiCl | 465.3 | 452.5 | 437.9 | 433.7 | 432.2 | 431.1 | 472.9 |
| NaCl | 394.6 | 394.5 | 379.6 | 381.6 | 384.8 | 387.7 | 407.4 |
| $Cl_2$ | 299.2 | 234.7 | 275.9 | 283.0 | 288.6 | 292.8 | 239.3 |
| HBr | 442.6 | 398.2 | 405.8 | 394.6 | 388.2 | 384.1 | 362.4 |
| LiBr | 425.9 | 400.5 | 401.8 | 397.1 | 394.5 | 392.5 | 425.1 |
| NaBr | 367.8 | 352.0 | 355.6 | 355.5 | 356.5 | 357.7 | 363.3 |
| FBr | 298.4 | 241.7 | 273.3 | 281.9 | 288.8 | 293.8 | 246.4 |
| $Br_2$ | 271.8 | 204.1 | 251.2 | 254.2 | 257.0 | 259.3 | 190.2 |
| $C_6H_6$ | 6341.0 | 5631.3 | 5758.8 | 5571.1 | 5444.0 | 5345.5 | 5463 |
| $C_4H_4O$ | 4627.8 | 4114.4 | 4125.6 | 4000.8 | 3923.2 | 3863.5 | 3977.4 |
| $C_4H_6$ | 4673.0 | 4236.9 | 4200.6 | 4052.4 | 3957.4 | 3884.8 | 3982 |
| $C_2H_6$ | 3354.3 | 3051.3 | 3038.8 | 2930.6 | 2860.0 | 2806.4 | 2787 |
| $N_2$ | 985.1 | 924.6 | 922.9 | 891.2 | 863.6 | 838.5 | 941.6 |
| $N_2H_4$ | 2128.9 | 1883.1 | 1892.8 | 1804.1 | 1742.3 | 1693.4 | 1696.4 |
| $H_2$ | 479.2 | 479.2 | 479.2 | 479.2 | 479.2 | 479.2 | 432.1 |
| $H_2O_2$ | 1241.7 | 1128.8 | 1108.4 | 1075.3 | 1054.9 | 1039.6 | 1055.5 |
| BeH | 261.6 | 238.7 | 240.2 | 230.7 | 224.0 | 218.6 | 216.8 |
| $BH_3$ | 1321.5 | 1223.7 | 1221.3 | 1179.7 | 1151.6 | 1129.8 | 1116.1 |
| $C_2H_2O_2$ | 2891.8 | 2615.8 | 2605.1 | 2534.3 | 2488.6 | 2452.4 | 2554.5 |
| $C_3H_4$ | 3257.8 | 2981.0 | 2933.1 | 2828.9 | 2761.4 | 2709.4 | 2806.1 |
| $C_4H_8$ | 5483.4 | 4878.0 | 4913.1 | 4733.7 | 4618.7 | 4531.9 | 4520.1 |
| $S_2$ | 457.3 | 413.4 | 443.9 | 454.7 | 463.4 | 470.3 | 421.6 |
| $SiH_4$ | 1524.6 | 1380.2 | 1435.2 | 1400.4 | 1376.1 | 1357.0 | 1265.9 |
| SiO | 761.1 | 738.3 | 713.8 | 716.1 | 719.3 | 721.4 | 794.1 |
| $SO_2$ | 1027.1 | 934.8 | 933.1 | 937.9 | 943.8 | 947.6 | 1062.9 |
| $O_2$ | 487.6 | 469.5 | 464.4 | 467.4 | 468.0 | 467.2 | 493.7 |
| CO | 1071.5 | 1036.7 | 1000.2 | 987.4 | 978.8 | 971.1 | 1071.8 |
| $CO_2$ | 1535.2 | 1457.0 | 1366.5 | 1346.1 | 1342.2 | 1341.2 | 1598 |
| $C_2H_2$ | 1823.8 | 1716.4 | 1657.3 | 1600.5 | 1562.3 | 1532.0 | 1626.5 |
| $Li_2$ | 92.2 | 72.8 | 69.8 | 57.9 | 48.7 | 41.0 | 100 |
| $CH_4$ | 1952.4 | 1815.4 | 1787.0 | 1725.2 | 1684.0 | 1652.3 | 1642 |
| $NH_3$ | 1392.8 | 1293.3 | 1260.1 | 1205.4 | 1167.7 | 1138.2 | 1157.9 |
| $H_2O$ | 1029.5 | 992.7 | 930.5 | 900.8 | 883.4 | 871.1 | 917.8 |
| MAE | 196.0 | 83.8 | 91.6 | 61.8 | 53.1 | 58.0 | |

$^{\dagger}$Reference [3]

**Table S8** Atomization energies of selected molecules (in kJ/mol) for OSIC($w$) with LSDA.

| System | OSIC($w$) | | | $E^{\dagger}_{Exp}$ |
|---|---|---|---|---|
| | $k=1$ | $k=2$ | $k=3$ | |
| HF | 590.4 | 585.6 | 584.1 | 566.6 |
| LiF | 549.1 | 547.7 | 548.0 | 575.6 |
| $F_2$ | 227.7 | 243.5 | 251.8 | 154.5 |
| HCl | 470.6 | 463.8 | 459.9 | 427.8 |
| LiCl | 456.5 | 453.8 | 452.8 | 472.9 |
| NaCl | 392.2 | 393.1 | 394.9 | 407.4 |
| $Cl_2$ | 293.3 | 295.0 | 296.4 | 239.3 |
| HBr | 422.7 | 414.8 | 409.9 | 362.4 |
| LiBr | 421.8 | 420.3 | 419.5 | 425.1 |
| NaBr | 369.0 | 369.7 | 370.8 | 363.3 |
| FBr | 302.9 | 308.6 | 312.8 | 246.4 |
| $Br_2$ | 269.1 | 269.7 | 270.4 | 190.2 |
| $C_6H_6$ | 6111.5 | 5998.9 | 5920.5 | 5463 |
| $C_4H_4O$ | 4402.7 | 4321.2 | 4269.9 | 3977.4 |
| $C_4H_6$ | 4442.8 | 4350.8 | 4291.5 | 3982 |
| $C_2H_6$ | 3190.8 | 3124.5 | 3080.8 | 2787 |
| $N_2$ | 977.4 | 961.2 | 944.2 | 941.6 |
| $N_2H_4$ | 2015.0 | 1960.8 | 1920.4 | 1696.4 |
| $H_2$ | 479.2 | 479.2 | 479.2 | 432.1 |
| $H_2O_2$ | 1179.1 | 1154.4 | 1138.2 | 1055.5 |
| BeH | 252.1 | 247.0 | 243.2 | 216.8 |
| $BH_3$ | 1268.3 | 1243.2 | 1225.9 | 1116.1 |
| $C_2H_2O_2$ | 2766.7 | 2718.9 | 2687.5 | 2554.5 |
| $C_3H_4$ | 3101.7 | 3036.7 | 2994.5 | 2806.1 |
| $C_4H_8$ | 5198.3 | 5086.7 | 5014.1 | 4520.1 |
| $S_2$ | 459.3 | 462.5 | 465.0 | 421.6 |
| $SiH_4$ | 1478.6 | 1459.8 | 1446.3 | 1265.9 |
| SiO | 758.0 | 759.5 | 760.9 | 794.1 |
| $SO_2$ | 1007.1 | 1005.9 | 1005.7 | 1062.9 |
| $O_2$ | 493.3 | 495.0 | 495.1 | 493.7 |
| CO | 1049.6 | 1040.9 | 1035.3 | 1071.8 |
| $CO_2$ | 1493.8 | 1489.6 | 1491.4 | 1598 |
| $C_2H_2$ | 1749.2 | 1713.8 | 1690.1 | 1626.5 |
| $Li_2$ | 81.7 | 77.2 | 74.0 | 100 |
| $CH_4$ | 1864.7 | 1827.9 | 1803.3 | 1642 |
| $NH_3$ | 1325.0 | 1292.1 | 1268.2 | 1157.9 |
| $H_2O$ | 974.2 | 953.3 | 941.0 | 917.8 |
| MAE | 144.6 | 122.5 | 107.5 | |

$^{\dagger}$Reference [3]

**Table S9** Barrier heights for BH6 set of data (in kcal/mol) for PZSIC, LSIC($z$), and LSIC($w$) methods.

| Reaction | Direction | PZSIC | LSIC($z$) | LSIC($w$) | | | | $E^{\dagger}_{Ref}$ |
|---|---|---|---|---|---|---|---|---|
| | | | $k=1$ | $k=1$ | $k=2$ | $k=3$ | $k=4$ | |
| $OH + CH_4 \rightarrow CH_3 + H_2O$ | Forward | 4.5 | 9.3 | 8.0 | 7.7 | 7.0 | 6.2 | 6.7 |
| | Reverse | 7.2 | 19.4 | 11.6 | 13.2 | 14.1 | 14.7 | 19.6 |
| $H + OH \rightarrow H_2 + O$ | Forward | 9.6 | 10.1 | 5.4 | 3.7 | 2.8 | 2.3 | 10.7 |
| | Reverse | 8.5 | 14.3 | 17.1 | 20.3 | 22.4 | 24.1 | 13.1 |
| $H + H_2S \rightarrow H_2 + HS$ | Forward | 1.9 | 2.3 | 3.0 | 3.0 | 2.9 | 2.9 | 3.6 |
| | Reverse | 10.3 | 19.5 | 19.9 | 22.4 | 23.8 | 24.7 | 17.3 |
| ME | | -4.8 | 0.7 | -1.0 | -0.1 | 0.3 | 0.6 | |
| MAE | | 4.8 | 1.3 | 3.6 | 4.6 | 5.0 | 5.5 | |

†Reference [4]

**Table S10** Barrier heights for BH6 set of data (in kcal/mol) for OSIC($w$) method.

| Reaction | Direction | OSIC($w$) | | | $E^{\dagger}_{Ref}$ |
|---|---|---|---|---|---|
| | | $k=1$ | $k=2$ | $k=3$ | |
| $OH + CH_4 \rightarrow CH_3 + H_2O$ | Forward | 4.4 | 3.8 | 3.2 | 6.7 |
| | Reverse | 7.9 | 7.7 | 7.7 | 19.6 |
| $H + OH \rightarrow H_2 + O$ | Forward | 7.2 | 5.9 | 5.2 | 10.7 |
| | Reverse | 13.7 | 16.1 | 17.8 | 13.1 |
| $H + H_2S \rightarrow H_2 + HS$ | Forward | 2.3 | 2.0 | 1.7 | 3.6 |
| | Reverse | 15.3 | 16.7 | 17.5 | 17.3 |
| ME | | -3.4 | -3.1 | -3.0 | |
| MAE | | 3.6 | 4.1 | 4.6 | |

†Reference [4]

**Table S11** Reaction energies for SIE11 set of data (in kcal/mol) for PZSIC, LSIC($z$), and LSIC($w$) methods.

| Reaction | PZSIC | LSIC($z$) | LSIC($w$) | | | | $E^{\dagger}_{Ref}$ |
|---|---|---|---|---|---|---|---|
| | | $k=1$ | $k=1$ | $k=2$ | $k=3$ | $k=4$ | |
| $He_2^+ \rightarrow He + He^+$ | 62.74 | 55.19 | 56.86 | 54.16 | 52.23 | 50.67 | 56.9 |
| $(NH3)_2^+ \rightarrow NH_3 + NH_3^+$ | 47.60 | 37.53 | 44.51 | 43.38 | 42.57 | 42.02 | 35.9 |
| $(H2O)_2^+ \rightarrow H_2O + H_2O^+$ | 45.65 | 40.07 | 49.64 | 51.20 | 51.67 | 51.86 | 39.7 |
| $C_4H_{10}^+ \rightarrow C_2H_5 + C_2H_5^+$ | 46.72 | 29.29 | 41.40 | 42.27 | 42.97 | 43.49 | 35.28 |
| $(CH3)_2CO^+ \rightarrow CH_3 + CH_3CO^+$ | 61.96 | 24.43 | 41.05 | 35.54 | 32.62 | 30.90 | 22.57 |
| $ClFCl \rightarrow ClClF^+$ | -3.61 | -3.36 | -6.52 | -8.15 | -9.18 | -9.96 | -1.01 |
| $C_2H_4...F_2 \rightarrow C_2H_4 + F_2$ | 0.85 | -1.74 | 0.39 | 0.75 | 1.04 | 1.27 | 1.08 |
| $C_6H_6...Li \rightarrow Li + C_6H_6$ | 19.69 | -4.00 | 13.18 | 7.69 | 3.48 | 0.31 | 9.50 |
| $NH_3...ClF \rightarrow NH_3 + ClF$ | 16.11 | 5.94 | 11.78 | 12.20 | 12.78 | 13.32 | 10.50 |
| $NaOMg \rightarrow MgO + Na$ | 98.36 | 81.01 | 83.58 | 79.30 | 77.16 | 75.88 | 69.56 |
| $FLiF \rightarrow Li + F_2$ | 89.54 | 93.18 | 71.60 | 65.48 | 62.66 | 60.93 | 94.36 |
| MAE | 11.51 | 4.31 | 8.28 | 8.30 | 8.81 | 9.27 | |

†Reference [5]

**Table S12** Reaction energies for SIE11 set of data (in kcal/mol) for OSIC($w$) method.

| Reaction | OSIC($w$) | | | $E^{\dagger}_{Ref}$ |
|---|---|---|---|---|
| | $k=1$ | $k=2$ | $k=3$ | |
| $He_2^+ \rightarrow He + He^+$ | 59.93 | 58.53 | 57.47 | 56.9 |
| $(NH_3)_2^+ \rightarrow NH_3 + NH_3^+$ | 48.88 | 49.29 | 49.47 | 35.9 |
| $(H_2O)_2^+ \rightarrow H_2O + H_2O^+$ | 52.25 | 54.11 | 54.87 | 39.7 |
| $C_4H_{10}^+ \rightarrow C_2H_5 + C_2H_5^+$ | 46.99 | 48.18 | 49.00 | 35.28 |
| $(CH_3)_2CO^+ \rightarrow CH_3 + CH_3CO^+$ | 50.57 | 47.76 | 46.10 | 22.57 |
| ClFCl $\rightarrow$ ClClF | -7.57 | -9.32 | -10.34 | -1.01 |
| $C_2H_4...F_2 \rightarrow C_2H_4 + F_2$ | 1.25 | 1.51 | 1.67 | 1.08 |
| $C_6H_6...Li \rightarrow Li + C_6H_6$ | 17.56 | 14.67 | 12.50 | 9.50 |
| $NH_3...ClF \rightarrow NH_3 + ClF$ | 16.14 | 16.61 | 16.87 | 10.50 |
| NaOMg $\rightarrow$ MgO + Na | 86.99 | 83.22 | 81.28 | 69.56 |
| FLiF $\rightarrow$ Li + $F_2$ | 78.02 | 74.18 | 72.48 | 94.36 |
| MAE | 11.13 | 11.03 | 10.86 | |

$^{\dagger}$Reference [5]

**Table S13** Dissociation energies for SIE4x4 set of data (in kcal/mol) for PZSIC, LSIC($z$), and LSIC($w$) methods.

| Reaction | $R/R_e$ | PZSIC | LSIC($z$) | LSIC($w$) | | | | $E^{\dagger}_{Ref}$ |
|---|---|---|---|---|---|---|---|---|
| | | | $k=1$ | $k=1$ | $k=2$ | $k=3$ | $k=4$ | |
| $H_2^+ \rightarrow H + H^+$ | 1.0 | 64.4 | 64.4 | 64.4 | 64.4 | 64.4 | 64.4 | 64.4 |
| | 1.25 | 58.9 | 58.9 | 58.9 | 58.9 | 58.9 | 58.9 | 58.9 |
| | 1.5 | 48.7 | 48.7 | 48.7 | 48.7 | 48.7 | 48.7 | 48.7 |
| | 1.75 | 38.2 | 38.2 | 38.2 | 38.2 | 38.2 | 38.2 | 38.3 |
| $He_2^+ \rightarrow He + He^+$ | 1.0 | 62.7 | 55.2 | 56.9 | 54.2 | 52.2 | 50.7 | 56.9 |
| | 1.25 | 48.8 | 44.2 | 45.4 | 43.9 | 42.7 | 41.8 | 46.9 |
| | 1.5 | 30.9 | 28.3 | 29.0 | 28.2 | 27.5 | 27.0 | 31.3 |
| | 1.75 | 17.5 | 16.1 | 16.5 | 16.1 | 15.7 | 15.4 | 19.1 |
| $(NH_3)_2^+ \rightarrow NH_3 + NH_3^+$ | 1.0 | 47.6 | 37.5 | 44.5 | 43.4 | 42.6 | 42.0 | 35.9 |
| | 1.25 | 33.3 | 32.6 | 39.0 | 39.5 | 39.0 | 38.4 | 25.9 |
| | 1.5 | 17.5 | 21.5 | 26.2 | 27.4 | 27.2 | 26.8 | 13.4 |
| | 1.75 | 8.4 | 11.6 | 13.7 | 14.1 | 13.9 | 13.5 | 4.9 |
| $(H_2O)_2^+ \rightarrow H_2O + H_2O^+$ | 1.0 | 45.7 | 40.1 | 49.6 | 51.2 | 51.7 | 51.9 | 39.7 |
| | 1.25 | 27.8 | 33.3 | 39.2 | 42.0 | 42.9 | 43.2 | 29.1 |
| | 1.5 | 14.4 | 18.4 | 20.0 | 21.3 | 21.9 | 22.2 | 16.9 |
| | 1.75 | 8.0 | 11.1 | 11.2 | 12.1 | 12.4 | 12.7 | 9.3 |
| MAE | | 3.0 | 2.6 | 4.7 | 5.5 | 5.8 | 5.9 | |

$^{\dagger}$Reference [6]

**Table S14** Dissociation energies for SIE4x4 set of data (in kcal/mol) for OSIC($w$) method (kcal/mol).

| Reaction | $R/R_e$ | OSIC($w$) | | | $E^{\dagger}_{Ref}$ |
|---|---|---|---|---|---|
| | | $k=1$ | $k=2$ | $k=3$ | |
| $H_2^+ \rightarrow H + H^+$ | 1.0 | 64.4 | 64.4 | 64.4 | 64.4 |
| | 1.25 | 58.9 | 58.9 | 58.9 | 58.9 |
| | 1.5 | 48.7 | 48.7 | 48.7 | 48.7 |
| | 1.75 | 38.2 | 38.2 | 38.2 | 38.3 |
| $He_2^+ \rightarrow He + He^+$ | 1.0 | 59.9 | 58.5 | 57.5 | 56.9 |
| | 1.25 | 47.3 | 46.5 | 45.9 | 46.9 |
| | 1.5 | 30.1 | 29.7 | 29.4 | 31.3 |
| | 1.75 | 17.1 | 16.9 | 16.7 | 19.1 |
| $(NH_3)_2^+ \rightarrow NH_3 + NH_3^+$ | 1.0 | 48.9 | 49.3 | 49.5 | 35.9 |
| | 1.25 | 39.9 | 41.6 | 42.2 | 25.9 |
| | 1.5 | 25.9 | 28.1 | 29.1 | 13.4 |
| | 1.75 | 13.5 | 15.1 | 15.8 | 4.9 |
| $(H_2O)_2^+ \rightarrow H_2O + H_2O^+$ | 1.0 | 52.3 | 54.1 | 54.9 | 39.7 |
| | 1.25 | 39.4 | 42.8 | 44.3 | 29.1 |
| | 1.5 | 20.1 | 22.0 | 22.9 | 16.9 |
| | 1.75 | 11.3 | 12.6 | 13.3 | 9.3 |
| MAE | | 5.2 | 6.0 | 6.4 | |

†Reference [6]

## References


1 S. J. Chakravorty, S. R. Gwaltney, E. R. Davidson, F. A. Parpia and C. F. p Fischer, *Phys. Rev. A*, 1993, **47**, 3649–3670.

2 A. Kramida, Yu. Ralchenko, J. Reader and NIST ASD Team, NIST Atomic Spectra Database (ver. 5.6.1), [Online]. Available: `https://physics.nist.gov/asd` [2018, July 25]. National Institute of Standards and Technology, Gaithersburg, MD., 2018.

3 National Institute of Standards and Technology, NIST Computational Chemistry Comparison and Benchmark Database NIST Standard Reference Database Number 101 Release 19, April 2018, Editor: Russell D. Johnson III `http://cccbdb.nist.gov/` DOI:10.18434/T47C7Z.

4 B. J. Lynch and D. G. Truhlar, *J. Phys. Chem. A*, 2003, **107**, 8996–8999.

5 L. Goerigk and S. Grimme, *J. Chem. Theory Comput.*, 2010, **6**, 107–126.

6 L. Goerigk, A. Hansen, C. Bauer, S. Ehrlich, A. Najibi and S. Grimme, *Phys. Chem. Chem. Phys.*, 2017, **19**, 32184–32215.
